# Supplementary material for: Data-Efficient Contrastive Language-Image Pretraining: Prioritizing Data Quality over Quantity
Source: arXiv:2403.12267 source file (2024-03-20)
Supplement: Supplementary file 1 [file proofs.tex]

\section{Full Derivation from Eq. \eqref{eq:cross_derivation:1} to Eq. \eqref{eq:cross_derivation:3}}\label{sec:proof:cross_derivation}

Let $\muuvv = \E_{i \in V} \ufnv^i$ and $\muulv = \E_{i \in V}\ufnl^i$ be the mean noisy shared features of images and captions in the full data $V$, respectively. Similarly, let $\muuvs = \E_{i \in S} \ufnv^i$ and $\muuls = \E_{i \in S} \ufnl^i$ be mean noisy shared features images and captions in the subset $S$. 

\begin{align}
& [\Crs]_{(k,k)} - [\Crv]_{(k,k)} = %\nonumber \\ 
% &
\frac{1}{|S|} \sum_{i \in S} \left[(\ufnv^i - \muuvs) \t{(\ufnl^i - \muuls)}\right]_{(k,k)} %\nonumber \\
% &
- \frac{1}{|V|} \sum_{j \in V} \left[(\ufnv^j - \muuvv) \t{(\ufnl^j - \muulv)}\right]_{(k,k)}.
\end{align}
\noindent Since the $(k,k)$-th element of $(\ufnv^j - \muuvv) \t{(\ufnl^j - \muulv)}$ is the same as the $(k,k)$-th element of $(\ufnl^j - \muulv) \t{(\ufnv^j - \muuvv)}$, we get
\begin{align}
[\Crs]_{(k,k)} - [\Crv]_{(k,k)} 
&= \frac{1}{|S|} \sum_{i \in S} \left[(\ufnv^i - \muuvs) \t{(\ufnl^i - \muuls)}\right]_{(k,k)} %\nonumber \\
% &
- \frac{1}{|V|} \sum_{j \in V} \left[(\ufnl^j - \muulv) \t{(\ufnv^j - \muuvv)}\right]_{(k,k)} \\
&%\hspace{2cm}
=\frac{1}{|V||S|} \sum_{i \in S} \sum_{j \in V} \Bigg[(\ufnv^i - \muuvs) \t{(\ufnl^i - \muuls)} %\nonumber \\ 
% &
- (\ufnl^j - \muulv) \t{(\ufnv^j - \muuvv)} \Bigg]_{(k,k)}. 
\end{align}
For the population data, the cross-covariance for underlying feature of latent class $k$ is entirely determined by examples in latent class $k$. Thus, we should only preserve the cross-covariance for underlying feature of latent class $k$, for examples in latent class $k$ in the full data and the subset $S$. 
\begin{align}
[\Crs]_{(k,k)} - [\Crv]_{(k,k)} 
&=\frac{1}{|V||S|} \sum_{i \in S_k} \sum_{j \in V_k} \Bigg[(\ufnv^i - \muuvs) \t{(\ufnl^i - \muuls)} %\nonumber \\ 
% &
- (\ufnl^j - \muulv) \t{(\ufnv^j - \muuvv)} \Bigg]_{(k,k)} \\
&=\frac{1}{|V||S|} \sum_{i \in S_k} \sum_{j \in V_k} \Bigg[\ufnv^i \t{\ufnl^i} - \ufnl^j\t{\ufnv^j} \Bigg]_{(k,k)} \nonumber \\
&~~~~ - \Bigg[\ufnv^i \t{\muuls} - \ufnl^j\t{\muuvv} \Bigg]_{(k,k)} - \Bigg[\muuvs \t{\ufnl^i} - \muulv \t{\ufnv^j} \Bigg]_{(k,k)} %\nonumber \\
% &
+ \Bigg[\muuvs \t{\muuls} - \muulv \t{\muuvv} \Bigg]_{(k,k)} \nonumber \\
&\hspace{-3.7cm}\text{Since the norm of all the vectors above is bounded by 1, we get} \nonumber\\
&\leq \frac{1}{|V||S|} \sum_{i \in S_k} \sum_{j \in V_k} \norm{\ufnv^i - \ufnl^j}\norm{\ufnl^i - \ufnv^j}  \nonumber \\ 
& \hspace{2cm}
+ \norm{\ufnv^i - \ufnl^j}\norm{\muuls - \muuvv} + \norm{\ufnl^i - \ufnv^j} \norm{\muuls - \muuvv} \\
&\leq \frac{1}{|V||S|} \sum_{i \in S_k} \sum_{j \in V_k} \norm{\ufnv^i - \ufnl^j} + \norm{\ufnl^i - \ufnv^j} %\nonumber \\
%&
+ \norm{\muuvs - \muulv} + \norm{\muuls - \muuvv} \\
&\leq \frac{1}{|V||S|} \Bigg( \sum_{i \in S_k}  \sum_{j \in V_k} \norm{\ufnv^i - \ufnl^j} + \norm{\ufnl^i - \ufnv^j} \Bigg)%\nonumber \\
% &
+ \underbrace{\norm{\muuvs - \muulv} + \norm{\muuls - \muuvv}}_{\text{cross-modal distance of means}}.
\end{align}
