# Supplementary material for: Data-Efficient Contrastive Language-Image Pretraining: Prioritizing Data Quality over Quantity
Source: arXiv:2403.12267 source file (2024-03-20)
Supplement: Supplementary file 2 [file old_proofs.tex]

\section{Proofs for Section \ref{sec:method}}\label{app:proof}

\subsection{Proof for Lemma \ref{lemma:subset_mmcl}}\label{app:proof:lemma:subset_mmcl}
\begin{proof}

\sj{I need to define the relation between $\pmms$ and $\pmm$ for $c$ to be meaningful.}

\sj{When we subset, we must renomralize our distribution so that the sum of probs of all image,caption pairs adds up to 1. $c$ is the renornmalizatoin constant. write this nicely}

Setting $c = \bigg({\sum_{\xv \in \Xv^S, \xl \in \Xl^S} \pmm(\xv, \xl)}\bigg)^{-1}$., we get:

\begin{align} &c^2 L_{SCL}^S + const. \\
&=  \underbrace{\sum_{\xv, \xl \in S} \bigg(\frac{c^2 \cdot \pmms(\xv, \xl)^2}{c^2 \cdot \pvs(\xv)\pls(\xl)} \bigg)}_{const} 
        -2c^2 \cdot \E_{\xv, \xl \in S} \fv{\xv}^\top \fl{\xl} + c^2 \cdot \E_{x_v^-, x_l^- \in S}\left(f_V(x_v^-)^\top f_L(x_l^-) \right)^2 \\
&=\sum_{\xv, \xl \in S}\bigg( \frac{c \cdot \pmms(x_v,x_l)}{\sqrt{c\cdot \pvs(x_v)} \sqrt{c \cdot \pls(x_l)}} - \sqrt{c \cdot \pvs(\xv)}\fv{\xv}^\top \sqrt{c \cdot \pls(\xl)}\fl{\xl} \bigg)^2 \\
&=\sum_{\xv, \xl \in S}\bigg( \frac{ \pmm(x_v,x_l)}{\sqrt{\pv(x_v)} \sqrt{\pl(x_l)}} - \sqrt{\pv(\xv)}\fv{\xv}^\top \sqrt{\pl(\xl)}\fl{\xl} \bigg)^2 \\
&= \norm{M_S \odot \tilde{A} - F_V F_L^\top}^2
\end{align}
\end{proof}

\subsection{Proof for \ref{lemma:errsv_bound}}\label{app:proof:lemma:errsv_bound}
\begin{proof}

\begin{align}
\errsv &:= \sigma_{k+1} - \sigma^S_{k+1} \\
&\leq \norm{\tilde{A} - M_S \odot \tilde{A}} \\
&= \sum_{\substack{\xv \in \Xv^S \\ \xl \notin \Xl^S}} \tilde{A}(\xv, \xl) + \sum_{\substack{\xv \notin \Xv^S \\ \xl \in \Xl}} \tilde{A}(\xv, \xl) + \sum_{\substack{\xv \notin \Xv^S \\ \xl \notin \Xl^S}} \tilde{A}(\xv, \xl) \\
&= \sum_{\substack{\xv \in \Xv^S \\ \xl \notin \Xl^S \\  y(\xv) = y(\xl)}} \tilde{A}(\xv, \xl) 
+ \sum_{\substack{\xv \in \Xv^S \\ \xl \notin Xl^S \\ y(\xv) \neq y(\xl)}} \tilde{A}(\xv, \xl) \nonumber \\
&+ \sum_{\substack{\xv \notin \Xv^S \\ \xl \in \Xl^S \\ y(\xv) = y(\xl)}} \tilde{A}(\xv, \xl)
+ \sum_{\substack{\xv \notin \Xv^S \\ \xl \in \Xl^S \\ y(\xv) \neq y(\xl)}} \tilde{A}(\xv, \xl) \nonumber \\
&+ \sum_{\substack{\xv \notin \Xv^S \\ \xl \notin \Xl^S \\ y(\xv) = y(\xl)}} \tilde{A}(\xv, \xl) + \sum_{\substack{\xv \notin \Xv^S \\ \xl \notin \Xl^S \\  y(\xv) \neq y(\xl)}} \tilde{A}(\xv, \xl) \\
&\leq \sum_{\substack{\xv \in \Xv^S \\ \xl \notin \Xl^S \\ y(\xv) = y(\xl)}} \tilde{A}(\xv, \xl) +  \sum_{\substack{\xv \notin \Xv^S \\ \xl \in \Xl^S \\ y(\xv) = y(\xl)}} \tilde{A}(\xv, \xl) + \sum_{\substack{\xv \notin \Xv^S \\ \xl \notin \Xl^S \\ y(\xv) = y(\xl)}} \tilde{A}(\xv, \xl) + \phi^y \\
&\leq \sum_{\substack{\xv \in \Xv^S \\ \xl \notin \Xl^S \\ y(\xv) = y(\xl)}} \tilde{A}(\xv, \xl) +  \sum_{\substack{\xv \notin \Xv^S \\ \xl \in \Xl^S \\ y(\xv) = y(\xl)}} \tilde{A}(\xv, \xl) + 2\cdot \sum_{\substack{\xv \notin \Xv^S \\ \xl \notin \Xl^S \\ y(\xv) = y(\xl)}} \tilde{A}(\xv, \xl) + \phi^y \\
&= \sum_{\substack{\xv \notin \Xv^S \\ \xl \in \Xv}} \tilde{A}(\xv, \xl) + \sum_{\substack{\xv \in \Xv \\ \xl \notin \Xv^S}} \tilde{A}(\xv, \xl) + \phi^y \\
&= \sum_{(\xv, \xl) \notin S} \bigg[ \sum_{\xl'} \tilde{A}(\xv, \xl') + \sum_{\xv'} \tilde{A}(\xv', \xl)\bigg] + \phi^y
\end{align}

Let $\cross((\xv, \xl)) = \sum_{\xl'} \tilde{A}(\xv, \xl') + \sum_{\xv'} \tilde{A}(\xv', \xl)$

Hence, 

\begin{align}
\errsv &\leq \sum_{(\xv, \xl) \notin S} \cross((\xv, \xl)) + \phi^y \\
&= \bigg(\sum_{(\xv, \xl) \in D} \cross((\xv, \xl)) - \sum_{(\xv, \xl) \in S} \cross((\xv, \xl))\bigg) +  \phi^y
\end{align}

Thus, we get the following bound on singular value error:

\begin{equation}\label{eq:errsv_bound}
\errsv \leq \sum_{(\xv, \xl) \in D} \cross((\xv, \xl)) - \sum_{(\xv, \xl) \in S} \cross((\xv, \xl)) +  \phi^y
\end{equation}

\end{proof}

\subsection{Proof for \ref{lemma:errc_bound}}\label{app:proof:lemma:errc_bound}

\begin{proof}

Let $\errc$ be the error in conductance 

\begin{equation}
    \errc := \phi^y_S - \phi^y
\end{equation}

By definition: 

\begin{align}
\phi^y_S &= \sum_{\xv \sim \Xv^S, \xl \sim \Xl^S} \pmms(\xv, \xl) \cdot \mathbbm{1}[y(\xv) \neq y(\xl)] 
\end{align}

We know by definition $\pmms(\xv, \xl) = c \pmm(\xv, \xl)$ where $c = \bigg({\sum_{\xv \in \Xv^S, \xl \in \Xl^S} \pmm(\xv, \xl)}\bigg)^{-1}$.

By definition, $\pmm(\xv, \xl) = A(\xv, \xl)$

\begin{align}
\phi^y_S &= c \sum_{\xv \sim \Xv^S, \xl \sim \Xl^S} A(\xv, \xl) \cdot \mathbbm{1}[y(\xv) \neq y(\xl)] \\
&= \frac{c}{2} \sum_{(\xv, \xl) \in S} \bigg( \sum_{\substack{\xl' \in \Xl^S \\ y(\xl') \neq y(\xv)}} A(\xv, \xl') + \sum_{\substack{\xv' \in \Xv^S \\ y(\xv') \neq y(\xl)}} A(\xv', \xl) \bigg) \\ 
&= \frac{c}{2} \sum_{(\xv, \xl) \in S} \bigg( (1 - \alpha^S_y) \sum_{y' \in [r] \setminus \{y(\xv) \}} \bigg(  \sum_{\substack{\xl' \in \Xl^S \\ y(\xl') = y'}} A(\xv, \xl') + \sum_{\substack{\xv' \in \Xv^S \\ y(\xv') = y'}} A(\xv', \xl) \bigg) \nonumber \\ &+ \alpha^S_y \bigg( \sum_{y' \in [r] \setminus \{y(\xv) \}} \sum_{\substack{\xl' \in \Xl^S \\ y(\xl') = y'}} A(\xv, \xl') + \sum_{y' \in [r] \setminus \{y(\xl) \}} \sum_{\substack{\xv' \in \Xv^S \\ y(\xv') = y'}} A(\xv', \xl) \bigg) \bigg) \\
&\leq \frac{1}{2} \sum_{(\xv, \xl) \in S} \bigg( (1 - \alpha^S_y) \sum_{y' \in [r] \setminus \{y(\xv) \}} \bigg(  \sum_{\substack{\xl' \in \Xl^S \\ y(\xl') = y'}} A(\xv, \xl') + \sum_{\substack{\xv' \in \Xv^S \\ y(\xv') = y'}} A(\xv', \xl) \bigg) \nonumber \\ &+ \alpha^S_y \bigg( \sum_{y' \in [r] \setminus \{y(\xv) \}} \sum_{\substack{\xl' \in \Xl^S \\ y(\xl') = y'}} A(\xv, \xl') + \sum_{y' \in [r] \setminus \{y(\xl) \}} \sum_{\substack{\xv' \in \Xv^S \\ y(\xv') = y'}} A(\xv', \xl) \bigg) \bigg) \\
&= \frac{c(1 - \alpha^S_y)}{2} \sum_{(\xv, \xl) \in S}   \sum_{y' \in [r] \setminus \{y(\xv) \}} \bigg(  \sum_{\substack{\xl' \in \Xl^S \\ y(\xl') = y'}} A(\xv, \xl') + \sum_{\substack{\xv' \in \Xv^S \\ y(\xv') = y'}} A(\xv', \xl) \bigg)  \nonumber \\
&+ \frac{c \alpha^S_y}{2} \sum_{(\xv, \xl) \in S} \bigg( \sum_{y' \in [r] \setminus \{y(\xv) \}} \sum_{\substack{\xl' \in \Xl^S \\ y(\xl') = y'}} A(\xv, \xl') + \sum_{y' \in [r] \setminus \{y(\xl) \}} \sum_{\substack{\xv' \in \Xv^S \\ y(\xv') = y'}} A(\xv', \xl) \bigg) \bigg) \\
&\leq \frac{(1 - \alpha^S_y)}{2} \sum_{(\xv, \xl) \in S}   \sum_{y' \in [r] \setminus \{y(\xv) \}} \bigg(  \sum_{\substack{\xl' \in \Xl^S \\ y(\xl') = y'}} A(\xv, \xl') + \sum_{\substack{\xv' \in \Xv^S \\ y(\xv') = y'}} A(\xv', \xl) \bigg) + \frac{\alpha^S_y}{2} \\
&\leq \frac{c}{2} \sum_{(\xv, \xl) \in S}   \sum_{y' \in [r] \setminus \{y(\xv) \}} \bigg(  \sum_{\substack{\xl' \in \Xl^S \\ y(\xl') = y'}} A(\xv, \xl') + \sum_{\substack{\xv' \in \Xv^S \\ y(\xv') = y'}} A(\xv', \xl) \bigg) + \frac{c \alpha^S_y}{2} \\
\end{align}

Hence,

\begin{equation}\label{eq:errc_bound}
    \errc \leq \sum_{(\xv, \xl) \in S} \Bigg[ \sum_{y' \in [r] \setminus \{y(\xv)\}} \divit{y'} + \divti{y'} \Bigg] - \phi^y
\end{equation}
\end{proof}

\subsection{Proof for \ref{lemma:erra_bound}}\label{app:proof:lemma:erra_bound}

\begin{proof}

\begin{align}
    \erra := \alpha^S_y - \alpha_y
\end{align}

\begin{align}
    \alpha^S_y = \E_{\xv, \xl \sim \pmms} \mathbbm{1}[y(\xv) \neq y(\xl)]\\
\end{align}

Assuming $Pr(y(\xv) \neq y(\xl)) \approx \pmm(\xv, \xl)$, we get: 

\begin{align}
    \alpha_y \approx \sum_{(\xv, \xl)} (1 - \pmm(\xv, \xl))
\end{align}

\begin{align}
    \erra &\approx \sum_{x \in S} (1 - \selfedge{x}) - \sum_{x \in D} (1 - \selfedge{x}) \\
    &= |S| - \sum_{x \in S} \selfedge{x} - - \sum_{x \in D} (1 - \selfedge{x})
\end{align}

Thus, we get the following bound on excess labeling error:

\begin{equation}\label{eq:erra_bound}
    \erra \approx |S| - \sum_{x \in S} \selfedge{x} - \sum_{x \in D} (1 - \selfedge{x})
\end{equation}
\end{proof}

\subsection{Proof for \ref{lemma:approx_errsv}}\label{proof:lemma:approx_errsv}

\sj{TODO}

\subsection{Proof for \ref{thm:error_bound}}\label{app:proof:thm:error_bound}

\begin{proof}

Using the bounds for $\errsv$, $\errc$ and $\erra$ from Lemmas \ref{lemma:errsv_bound}, \ref{lemma:errc_bound} and \ref{lemma:erra_bound} respectively, we have:

\begin{align}
\err(S) &\leq \underbrace{\sum_{(\xv, \xl) \in D} \cross((\xv, \xl)) - \sum_{(\xv, \xl) \in S} \cross((\xv, \xl)) +  \phi^y}_{\errsv} \nonumber \\ 
&+ \underbrace{\sum_{(\xv, \xl) \in S} \Bigg[ \sum_{y' \in [r] \setminus \{y(\xv)\}} \divit{y'} + \divti{y'} \bigg] - \phi^y}_{\errc} \nonumber \\
&+ \underbrace{|S| - \sum_{x \in S} \selfedge{x} - \sum_{x \in D} (1 - \selfedge{x})}_{\erra}
\end{align}

Simplifying and dropping terms not dependent on $S$ and since $|S|$ is fixed, we get: 

\begin{equation}
    S_* \approx \argmin_S \Bigg[ -1 \cdot \sum_{(\xv, \xl) \in S} \bigg(\cross((\xv, \xl))  
    +  \selfedge{x}
    - \sum_{y' \in [r] \setminus \{y(\xv)\}} \divit{y'} + \divti{y'} \bigg)
    \Bigg]
\end{equation}
\end{proof}


\subsection{Proof for \ref{remark:simple_obj}}\label{app:proof:remark:simple_obj}

\sj{TO DO}

\subsection{Proof for \ref{thm:gen_gap}}\label{app:proof:thm:gen_gap}

linear probe proof in ipad. for $v\setminus s$, say we assume that prediction is approximately average of predicttions on S, scaled by similarity. then cause of bounds b1 and b2 we should be good. 

zs proof sketch: 

$Pr(x \in S)$ correctly classified
\begin{proof}
\end{proof}
